# Supplementary material for: Disordered Zero-Index Metamaterials Based On Metal Induced Crystallization
Source: arXiv:1901.10379 ancillary file (2019-01-29)
Supplement: Supplementary file 1 [file Supplementary_Information.pdf]

# Supplementary Information for:
# Disordered Zero-Index Metamaterials Based On Metal Induced Crystallization

Henning Galinski[1], Andreas Wyss[1], Mattia Seregni[1], Huan Ma[1], Volker Schnabel[1], Alla Sologubenko[1,2], & Ralph Spolenak[1]

[1]*Laboratory for Nanometallurgy, ETH Zurich, Zurich, Switzerland*

[2]*Scientific Center for Optical and Electron Microscopy, ETH Zurich, Zurich, Switzerland*

## Effective Medium Approximation

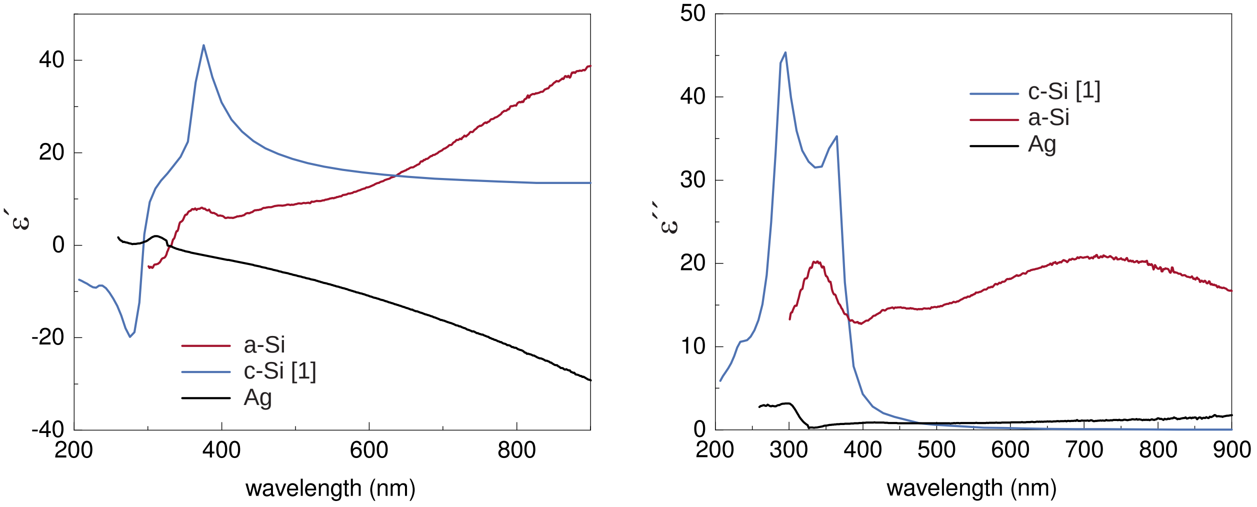


**Figure S1** – Real ($\epsilon'$) and imaginary ($\epsilon''$) part of the single components of the Ag-Si metal-semiconductor composite. Ag and and amorphous silicon (a-Si) have been measured using ellipsometry, while data from literature [1] have been used for crystalline silicon (c-Si)). It can be seen that from 300 to 340nm, the condition for suppressed scattering [2,3], i.e. ($\epsilon_{\text{core}} < \epsilon_{\text{medium}} < \epsilon_{\text{shell}}$) is fulfilled. Here, $\epsilon_{\text{core}}$ corresponds to a-Si, $\epsilon_{\text{medium}}$ to Ag and $\epsilon_{\text{shell}}$ to c-Si.

Here, we evaluate the concept of metal induced crystallization in immiscible metal-semiconductor composites to design ENZ materials with configurable $\epsilon' \approx 0$ states for two semiconducting materials, namely silicon (Si) and germanium. Using a simple effective medium model ([4]) we derive the near-zero phase diagrams. The complex permittivity of metal-semiconducting composites for a given composition $f$ is given by,

$$\epsilon_{\text{eff}}(\lambda, r_1, r_2, f) = \epsilon_{\text{Metal}}(\lambda)\frac{f \cdot (\epsilon_{\text{Core-Shell}}(\lambda, r_1, r_2) - \epsilon_{\text{Metal}}(\lambda) + \epsilon_{\text{Core-Shell}}(\lambda, r_1, r_2) + \epsilon_{\text{Metal}}(\lambda))}{f \cdot (\epsilon_{\text{Metal}}(\lambda) - \epsilon_{\text{Core-Shell}}(\lambda, r_1, r_2) + \epsilon_{\text{Core-Shell}}(\lambda, r_1, r_2) + \epsilon_{\text{Metal}}(\lambda))}. \tag{1}$$

Thereby the effective permittivity of the core-shell $\epsilon_{\text{Core-Shell}}$ is given by [5],

$$\epsilon_{\text{Core-Shell}}(\lambda, r_1, r_2) = \epsilon_{\text{Shell}}(\lambda)\frac{2 * \epsilon_{\text{Shell}}(\lambda) + \epsilon_{\text{Core}}(\lambda) + 2 * (r_1/(r_2))^3(\epsilon_{\text{Core}}(\lambda) - \epsilon_{\text{Shell}}(\lambda))}{2 * \epsilon_{\text{Shell}}(\lambda) + \epsilon_{\text{Core}}(\lambda) - 2 * (r_1/(r_2))^3(\epsilon_{\text{Core}}(\lambda) - \epsilon_{\text{Shell}}(\lambda))}, \tag{2}$$

where $r_1$ and $r_2$ are the inner and outer radius of the core-shell particle. The permittivity of the single components has been determined using ellipsometry in case of Ag and a-Si (see Fig.S1) and a-Ge.

### Ag-Si system

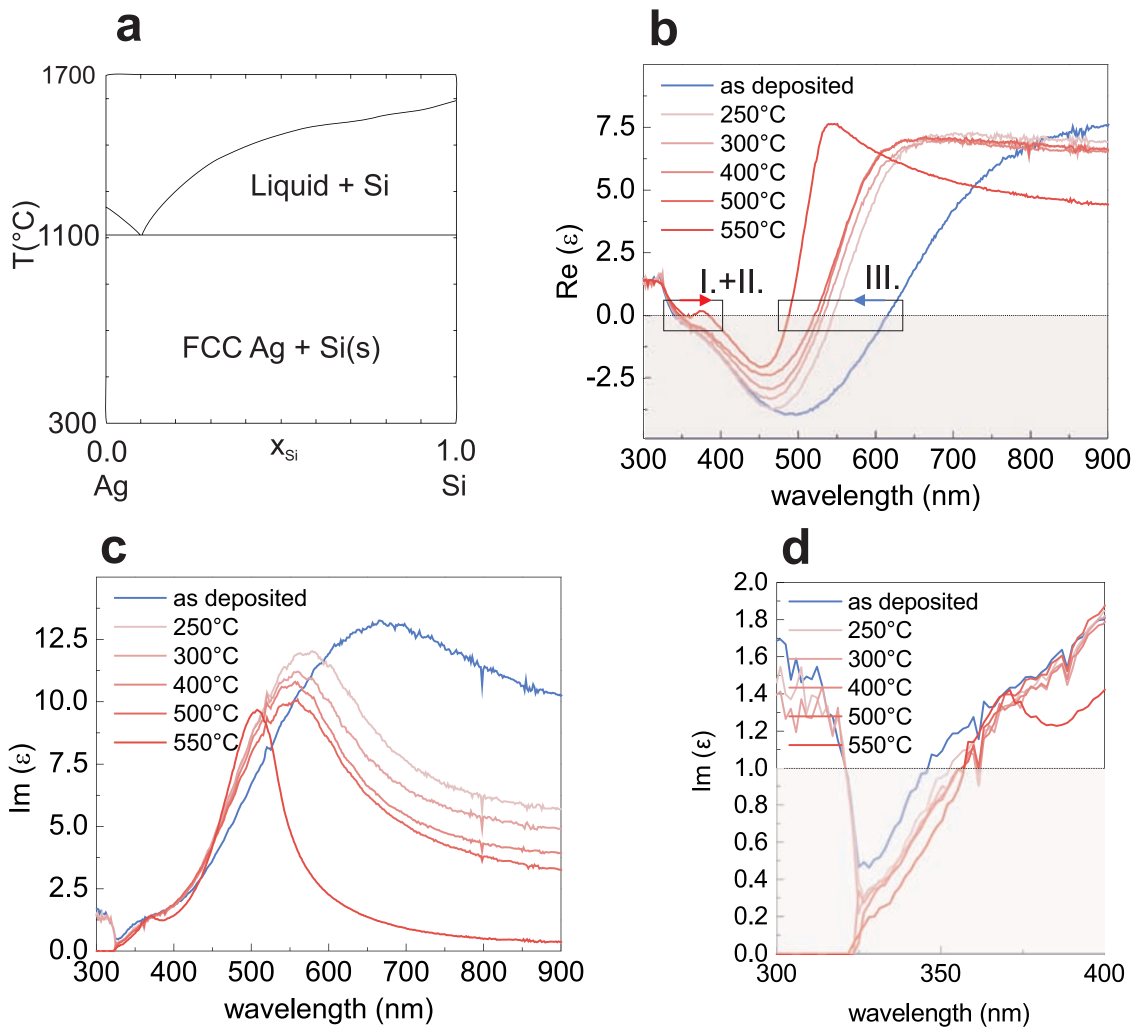


**Figure S2** – (a) Thermodynamic phase diagram of the immiscible Ag-Si system. (b) Real and (c) imaginary part of the dielectric function of $Ag_{.55}Si_{.45}$ as function of thermal treatment. Panel (d) shows a zoomed-in view of imaginary part of the dielectric function of $Ag_{.55}Si_{.45}$.

**Ag-Ge system**

In case of Ag-Ge, a phase analysis was performed, on some of the composites produced, by X-ray diffraction (XRD) with an X'Pert Pro diffractometer from PANalytical using Cu-$K_\alpha$ radiation ($\lambda = 1.54 \cdot 10^{-10}$ m). $\theta - 2\theta$ scans were acquired within a range of 20-90 and a step size of 0.0525. Raman spectroscopy was carried out in order to estimate the crystallinity of the differently annealed mixtures. The measurements were performed on a WITec Alpha 300 confocal Raman system with 532 nm excitation. The device featured a 100x objective lens with numerical aperture NA = 0.9 (Nikon Plan) and a fibercoupled grating spectrometer (2400 lines/mm) giving a spectral sampling resolution of 0.7 $cm^{-1}$. A laser power as low as 760 $\mu$W was used in order to avoid laser induced crystallization of the semiconductor. Transmission electron microscopy (TEM) was performed on the AD state of the mixture $Ag_{38}Ge_{62}$ to analyze microstructure and phases within the film. An FEI Tecnai F30 instrument, operated at 300kV was used for the bright/dark field imaging and the selected area diffraction study.

Transmission electron microscopy (TEM) of the as-deposited Ag-Ge systems confirmed a metastable nature of this material. Figure S3d shows a bright-field image depicting the amorphous Ge-Ag matrix with some dilute Ag-enriched nuclei. An increase in crystallinity and Ag NCs size were verified with Raman spectroscopy and x-ray diffraction shown in Fig. S3f and Fig. S3g respectively. The optical properties, in terms of permittivity, have been determined using ellipsometry. Figure S4(a) presents the effect on the real permittivity of this nano-materials upon compositional changes. The spectra can be subdivided in two regions with characteristic ZI behavior (Fig. S4a). Region I corresponds to the known Drude-Lorentz response of silver [6,] . This feature is only weakly

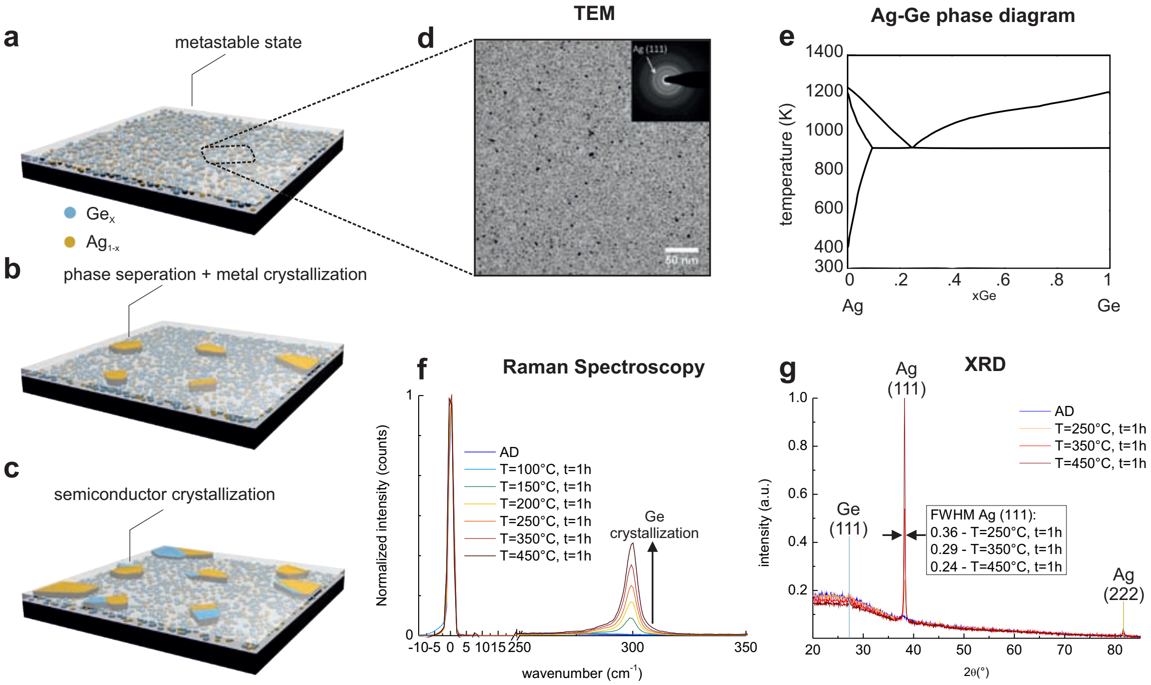


**Figure S3** – ENZ Materials by metal induced crystallization. (a)-(c) Different regimes of a quasi-immiscible $Ag_xGe_{1-x}$ starting from a "quasi-amorphous" solid solution after deposition (a), phase separation and formation of nanocrystalline metal crystallites after low temperature annealing (b), metal induced crystallization of the germanium phase after medium temperature annealing (c). (d) TEM bright field image of an as-deposited $Ag_{.38}Ge_{.62}$ thin film showing dilute Ag-enriched nuclei (dark spots) embedded in an amorphous matrix (brighter region). Panel (e) shows the thermodynamic phase diagram of the quasi-immiscible Ag-Ge system. (f) Raman spectra of $Ag_{.38}Ge_{.62}$ thin films in different annealing states. The peak at a wavenumber of 300 cm$^{-1}$ corresponds to crystalline Ge. (g) XRD pattern of $Ag_{.38}Ge_{.62}$ thin films in different annealing states. The inset reports the FWHM of the Ag(111) peak indicating growth of the silver phase with increasing temperature.

dependent on compositional changes and characterized by a red-shift of the critical ZI wavelength once the silver fraction is smaller than $50\%$ (Fig.S4b). A fraction of $50\%$ also coincides with the percolation threshold of a $2D$ system, a common assumption for thin films. In region II the spectra show a rich dynamical scenario as the metal content is varied. The critical wavelength given by $Re(\epsilon) \approx 0$ is continuously red-shifted to higher wavelength as the metal content is increased, see also Fig.S4b. The situation abruptly changes for a metal content of $42\%$ and a broadband ZI feature emerges spanning from $600$ to $1000$ nm. A similar behaviour of the permittivity is observed for

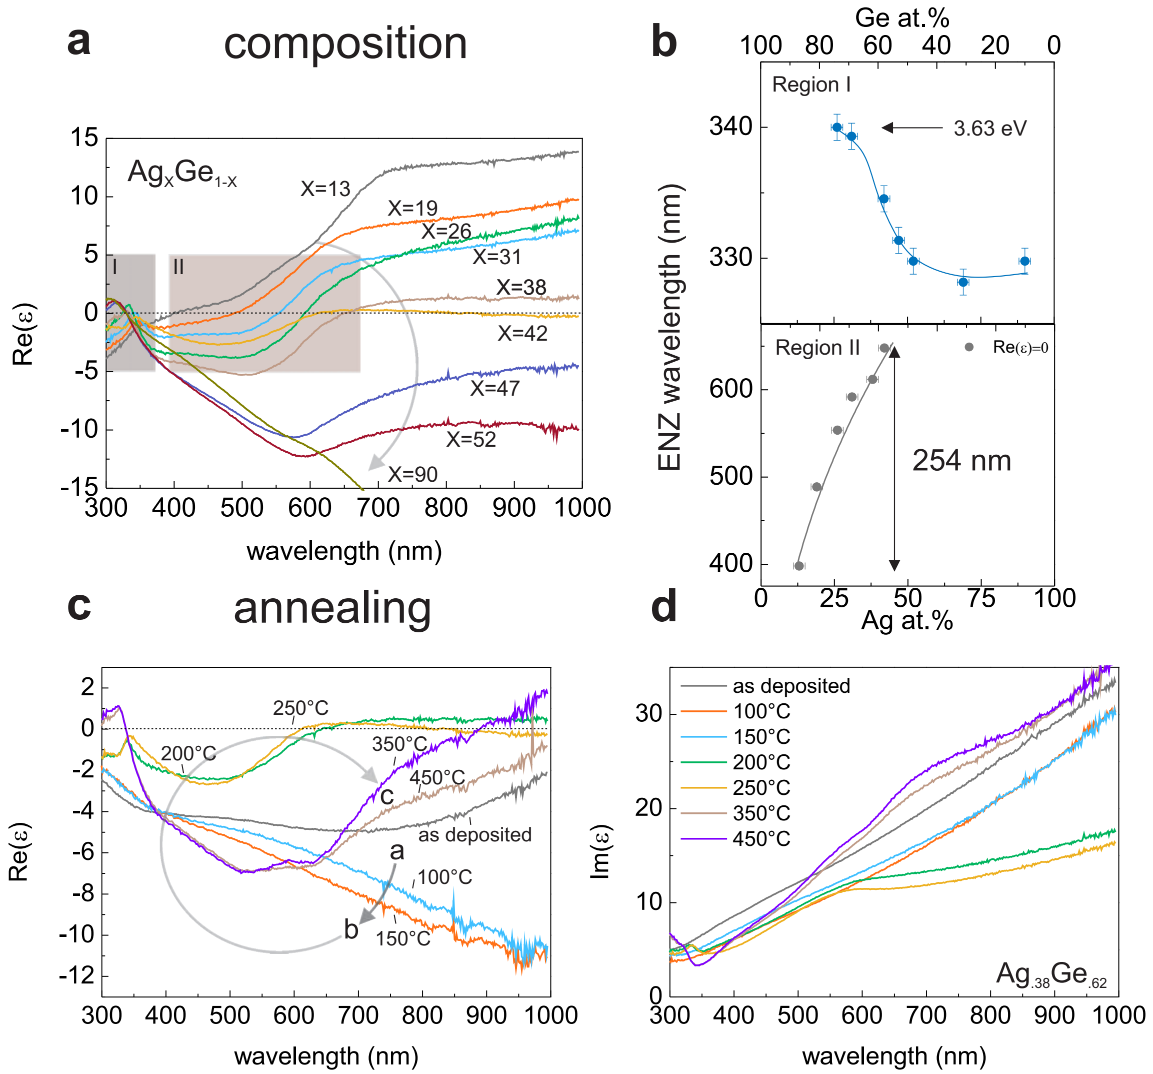


**Figure S4** – Optical properties of ENZ Materials by "metal induced crystallization. (a) Configurable $Re(\epsilon) \approx 0$ condition for $Ag_xGe_{1-x}$ composites as function of metal content. All spectra correspond to an annealing state of 250°C,1h. Panel (b) shows the compositional dependence of the two ENZ features in the spectra. (c)-(d) Real and imaginary part of the dielectric function of $Ag_{.38}Ge_{.62}$ as function of thermal treatment. The annealing state of 250°C shows a broad $Re(\epsilon) \approx 0$ region. Letters a,b,c in panel (c) correspond to the different thermodynamic states as illustrated in Fig.S3(a-c).

increasing annealing temperature for a given composition, shown in Fig. S4(d). Above a critical temperature of 200°C the ZI feature red-shifts with increasing temperature, suggesting that annealing can be used to configure materials with different ZI transitions. However, it has to be noted

that the losses (Fig. S4d), represented by the imaginary part of the permittivity $Im(\epsilon)$, within the designed materials are still to high to allow for ZI behavior. This effect is mostly due to the presence of amorphous Ge, characterized with high intrinsic losses with respect to its crystalline phase.

### Finite-Element Method Simulations

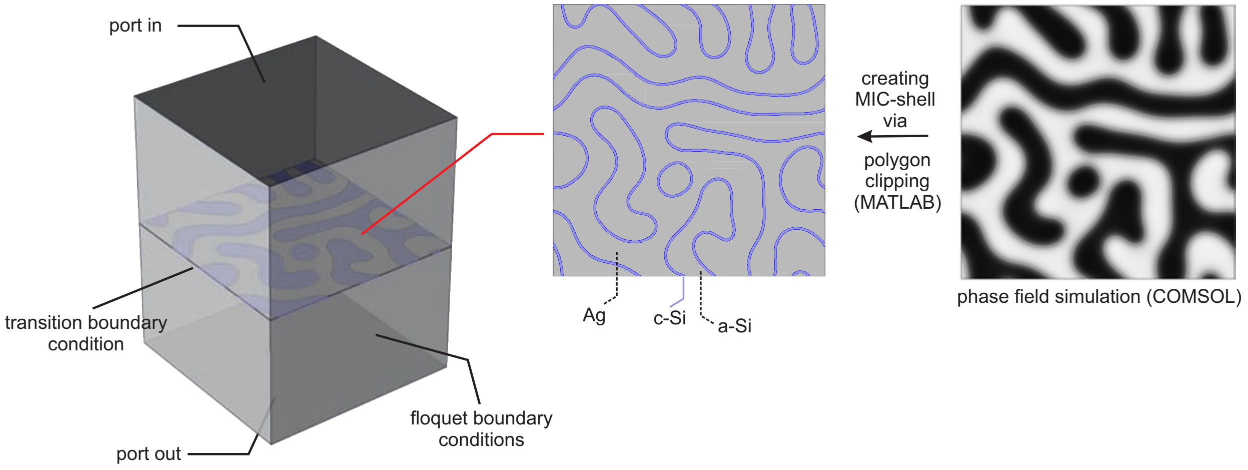


**Figure S5** – Illustration of the three-dimenssional FEM model with used boundary and port conditions. The MIC-based zero-index material is modelled using a phase-separated composite produced via COMSOL Multiphysics' phase-field package and Matlab.

The electromagnetic response to a monochromatic excitation of these near-zero materials is modelled using COMSOL Multiphysics. Figure S5 reports the used three-dimensional simulation setup which imposes periodicity in the x and y direction. The zero-index material is modelled using a phase-separated composite produced via COMSOL Multiphysics' phase-field package. To add the conformal crystalline Si shell, the polygons of the amorphous Si phase are exported to Matlab where from the existing set of polygons a new set of polygon, outset/inset by distance $\Delta$, is created. Based on STEM images, the zero-index material can be considered two-dimensional, which

allow us to use a transition boundary in the simulation with numerically defined thickness, rather than a geometrically extended layer.


1. Aspnes, D. E. and Studna, A. A. *Phys. Rev. B* **27**, 985–1009 Jan (1983).

2. Kerker, M. *J. Opt. Soc. Am.* **65**(4), 376–379 Apr (1975).

3. Kerker, M. *Aerosol Science and Technology* **1**(3), 275–291 (1982).

4. Levy, O. and Stroud, D. *Phys. Rev. B* **56**, 8035–8046 Oct (1997).

5. Chettiar, U. K. and Engheta, N. *Opt. Express* **20**(21), 22976–22986 Oct (2012).

6. Yang, H. U., D'Archangel, J., Sundheimer, M. L., Tucker, E., Boreman, G. D., and Raschke, M. B. *Phys. Rev. B* **91**, 235137 (2015).
